# Supplementary material for: Janus spectra in two-dimensional flows
Source: arXiv:1608.03407 ancillary file (2016-08-11)
Supplement: Supplementary file 1 [file janus_spectra_supp1.pdf]

# Supplemental Material:
# Janus spectra in two-dimensional flows

Chien-Chia Liu, Rory T. Cerbus, and Pinaki Chakraborty

*Fluid Mechanics Unit, Okinawa Institute of Science and Technology Graduate University, Onna-son, Okinawa, Japan 904-0495*

## S-1. DECAYING 2D TURBULENCE IN AN ATMOSPHERIC FLOW

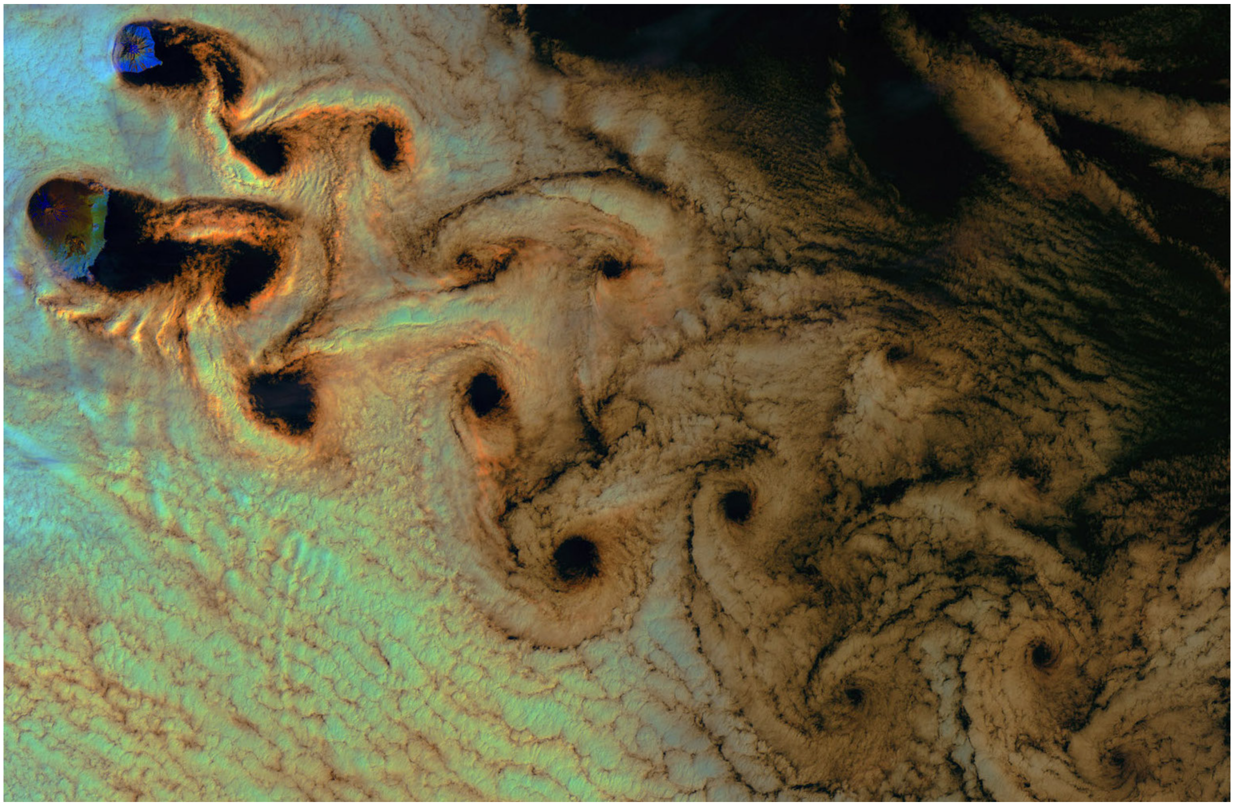

FIG. S-1. Quasi-2D turbulent flow of wind over Alaska's Aleutian Islands. The islands shed eddies as the wind sweeps past them. The eddies, made visible by the clouds, render the flow turbulent. The mean flow is directed from top–left to bottom–right of the image. This satellite image was acquired by the Landsat mission; http://landsat7.usgs.gov/

## S-2. ERROR BARS IN THE ENERGY SPECTRA

The shaded regions in Figs. 2d, 3c, 3f, S-2a, S-3a, and S-4a represent error bars. There are two contributions to the error bars, $dE(k)$ (see [1, 2] for details):

First, from the statistical fluctuations of the velocity series. We chop the velocity series into $N$ equally sized windows and treat them as independent realizations. The ensemble fluctuations about the ensemble average give an estimate of the statistical uncertainty:

$$dE(k) = \frac{\sigma(E(k))}{\sqrt{N}}, \tag{S-1}$$

where $\sigma$ is the standard deviation.

The second contribution comes from the random-in-time sampling of Laser Doppler Velocimetry (LDV). Frequencies higher than the mean sampling frequency are in principle measurable (not subject to a Nyquist limitation), but not well resolved. As shown in [2], this has two effects on the calculated spectrum $E_I(k)$:

$$E_I(k) = \frac{1}{1 + k^2/f_s^2}\left[E(k) + \frac{2\sigma_u^2}{f_s^3/\lambda^2}\right]. \tag{S-2}$$

where $E(k)$ is the "true" spectrum of the velocity field, $f_s$ is the mean sampling frequency, $\sigma_u$ is the r.m.s. velocity, and $\lambda$ is the Taylor microscale. The first multiplicative term is like a low pass filter with a cutoff frequency set by $f_s$. The additive term is a white noise contribution stemming from the random sampling times. Rearranging eq. S-2, we estimate the uncertainty in the interpolated $E_I(k)$ as:

$$dE(k) = |E(k) - E_I(k)| \approx \frac{2\sigma_u^2}{f_s^3/\lambda^2} + \frac{E_I(k)k^2}{f_s^2}. \tag{S-3}$$

## S-3. ADDITIONAL CASES OF THE JANUS SPECTRA

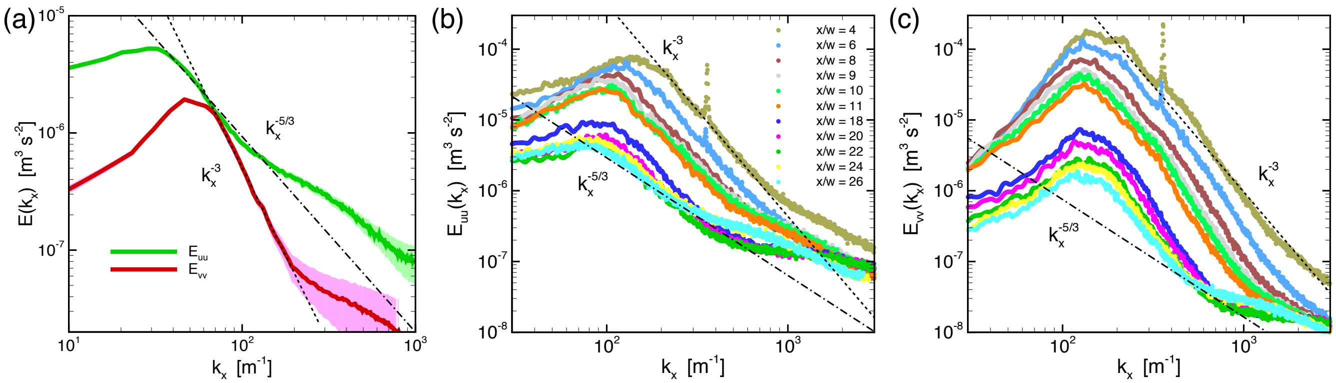


FIG. S-2. Janus spectra in turbulence induced by two rods. The soap film (w = 15 mm) is pierced with two rods (of diameters 1.5 mm and 2 mm; the first is placed 13 mm transversely away from the centerline; the second is placed 12 mm transversely away from the centerline and 90 mm below the first.) The mean velocity at the centerline ranges from 2.25 m/s to 2.60 m/s. (a) Janus spectra at $x/w = 26$. (b, c) Evolution of $E_{uu}(k_x)$ and $E_{vv}(k_x)$ with downstream distance. All measurements reported in the supplementary material are along the centerline of the channel and are well upstream ($> 15w$) of the Marangoni shock.

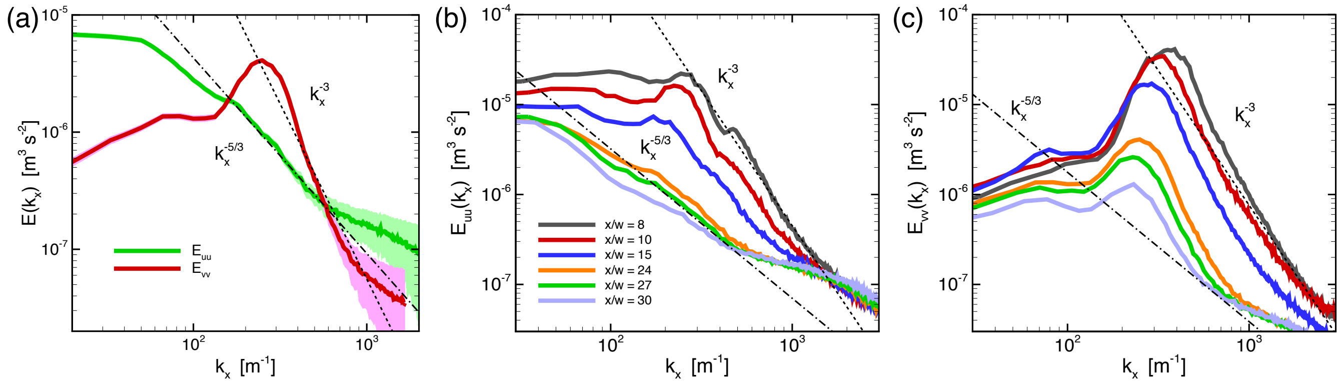


FIG. S-3. Janus spectra in turbulence induced by one rod. The soap film (w = 10 mm) is pierced at the centerline with a rod of diameter 0.5 mm. The mean velocity at the centerline ranges from 2.10 m/s to 2.40 m/s. (a) Janus spectra at $x/w = 24$. (b, c) Evolution of $E_{uu}(k_x)$ and $E_{vv}(k_x)$ with downstream distance.

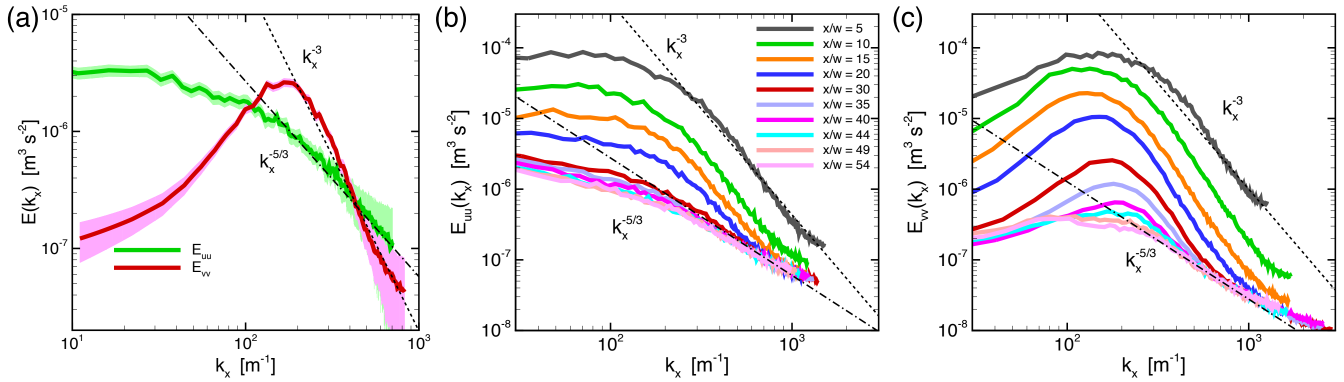


FIG. S-4. Janus spectra in turbulence induced by a comb. The soap film (w = 8 mm) is pierced symmetrically about the centerline with a comb (which consists of three rods, each of diameter 1.5 mm, spaced 2 mm apart from each other). The mean velocity at the centerline ranges from 1.57 m/s to 2.55 m/s. (a) Janus spectra at $x/w = 30$. (b, c) Evolution of $E_{uu}(k_x)$ and $E_{vv}(k_x)$ with downstream distance.

## S-4. TURBULENT VORTICITY AND MEAN SHEAR

In Fig. 2e in the manuscript, we plot the evolution of turbulent vorticity ($\omega$) and mean shear ($S$) with downstream distance.

Following [3], we estimate the turbulent vorticity at the centerline, $\omega$, from the decay of the turbulent kinetic energy, $e \equiv < u^2/2 + v^2/2 >$, where $<>$ represents the ensemble

average. For 2D, homogeneous, isotropic turbulence [4]:

$$\frac{de}{dt} = -\nu\omega^2, \tag{S-4}$$

where $t$ is the time and $\nu$ is the kinematic viscosity of the fluid. In soap-film channels (and in experiments of grid turbulence in general), the analog of decay in $t$ is the decay in $x$. Here the time is the "transit time" [5]: $t = \int dx/U$. From LDV data we compute $de/dt$, and use eq. S-4 to estimate $\omega$.

Now consider the mean shear. Note that although the mean shear is negligible at the centerline, the eddies that contribute to the energy spectra are affected by the mean shear from across the width of the channel. To approximate the mean shear across the width of the channel, $S$, at any given location $x$, we estimate $S \approx U/(w/2)$, where $U$ is the mean velocity at the centerline at $x$ and $w$ is the width of the soap-film channel (see Fig. 2a).

## S-5. ENERGY FLUX

Following [6], we estimate the energy flux from the time evolution of the energy spectra. Because the turbulent kinetic energy equation can be split into separate evolution equations for $u^2$ and $v^2$, we can compute the energy flux for the $u$ component, $\Pi_{uu}(k_x)$, from the evolution of $E_{uu}(k_x)$, and the energy flux for the $v$ component, $\Pi_{vv}(k_x)$, from the evolution of $E_{vv}(k_x)$.

Invoking the concept of the transit time (see above), we consider the evolution of $E_{uu}(k_x, t)$. (Similar considerations also apply to $E_{vv}(k_x, t)$.) $E_{uu}(k_x, t)$ changes with time because of the decay of the turbulent kinetic energy and because of the transfer of energy between scales. To focus on this transfer, instead of $E_{uu}(k_x, t)$, we consider the evolution of $E_{uu}(k_x, t)/u^2_{\rm rms}(t)$, where $u^2_{\rm rms}(t) \equiv \int_0^\infty E_{uu}(k_x, t) dk_x$. We approximate the energy transfer function as $T_{uu}(k_x, t) \approx u^2_{\rm rms}(t)\partial(E_{uu}(k_x, t)/u^2_{\rm rms}(t))/\partial t$. The energy flux function can be expressed as:

$$\Pi_{uu}(k_x, t) = \int_0^{k_x} T_{uu}(\tilde{k}_x, t) d\tilde{k}_x. \tag{S-5}$$

Negative $\Pi_{uu}(k_x, t)$ indicates that the energy is transferred from smaller to larger scales, i.e., an inverse flux.

For turbulence induced by a comb, we compute $\Pi_{uu}(k_x)$ and $\Pi_{vv}(k_x)$ at different downstream locations (Fig. S-5). We focus attention to the inertial range, which we identify using

the energy spectra. Note that both $\Pi_{uu}(k_x)$ and $\Pi_{vv}(k_x)$ are negative. Further, as the flow evolves from $\alpha_u \approx \alpha_v \approx 3$ to $\alpha_u \approx 5/3$ and $\alpha_v \approx 3$, the inverse energy flux is preferentially enhanced for the $u$ component, as can be inferred by comparing $\Pi_{uu}(k_x)$ and $\Pi_{vv}(k_x)$.

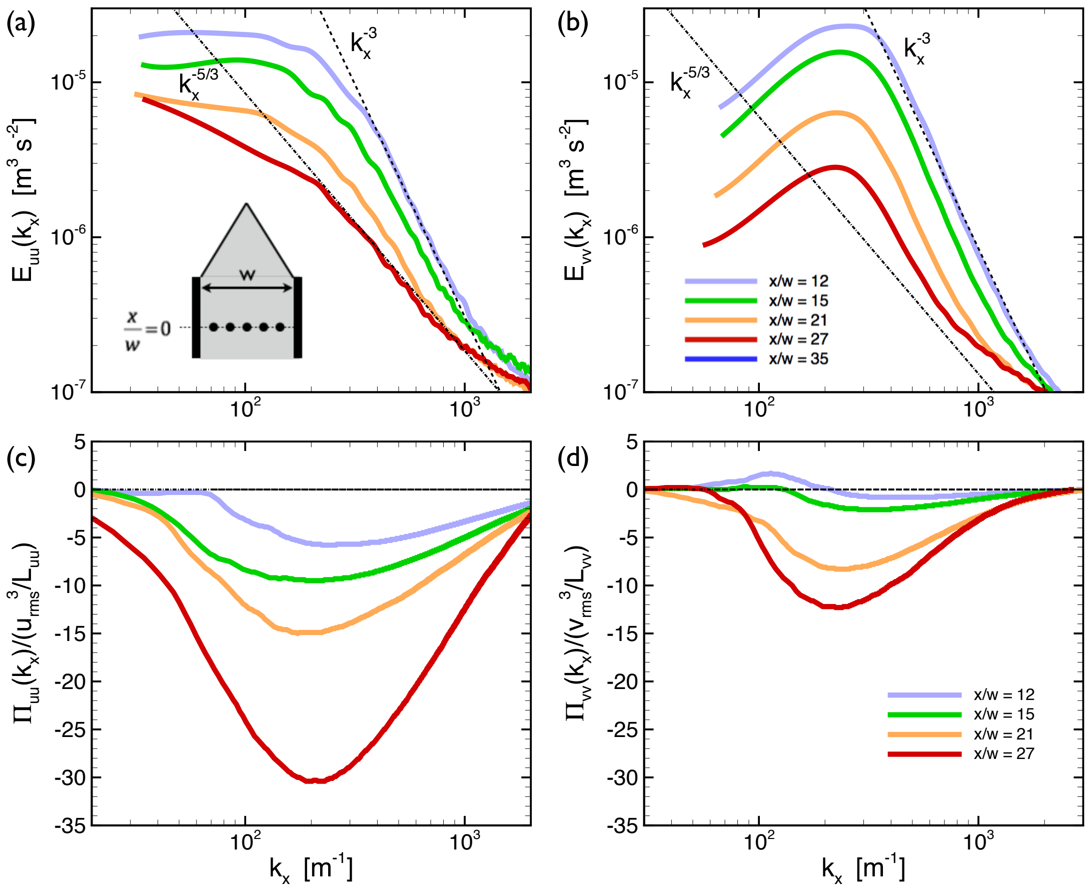


FIG. S-5. Energy flux in turbulence induced by a comb (see Fig. 3 d–f). (a, b) Evolution of $E_{uu}(k_x)$ and $E_{vv}(k_x)$. (c, d) Evolution of $\Pi_{uu}(k_x)$ and $\Pi_{vv}(k_x)$. We non-dimensionalize $\Pi_{uu}(k_x)$ by $u_{\rm rms}^3/L_{uu}$, where $L_{uu}$ is a large scale for the $u$ component, $L_{uu} = u_{\rm rms}^2/\int_0^\infty k_x E_{uu} dk_x$. Similarly, we non-dimensionalize $\Pi_{vv}(k_x)$.

As an aside we make two comments. First, in the span of wavenumbers where $E_{uu}(k_x) \sim k_x^{-5/3}$, $\Pi_{uu}(k_x)$ is negative but is not a constant. This is typical for experimental and computational data: the inverse energy cascade is clearly discernible in $E(k)$, but the attendant $\Pi(k)$ is not constant; see, e.g., Fig. 5 in [4]. Second, in the region not far downstream of the comb ($x/w \lesssim 15$)—the region of direct enstrophy cascade, $\alpha_u \approx \alpha_v \approx 3$—$\Pi_{uu}(k_x)$ and $\Pi_{vv}(k_x)$ are small but negative in the inertial range. That is, there is a small inverse flux

of energy in the region of direct enstrophy cascade. This is consistent with the experiments reported in [7].

## S-6. FLOW VISUALIZATION

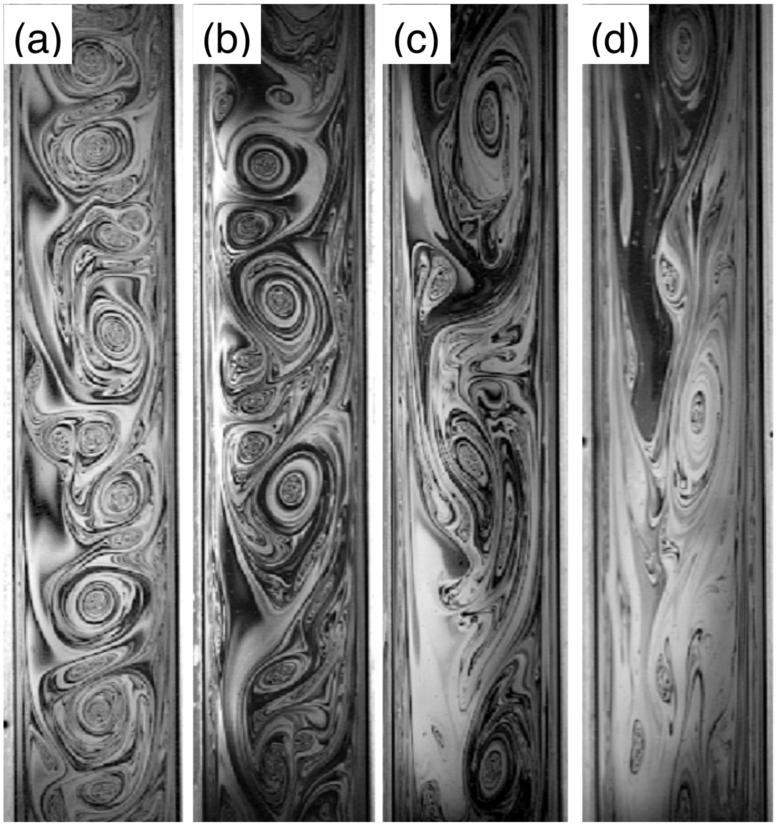


FIG. S-6. Turbulent eddies distorted by the sheared mean flow. The soap film (w = 22 mm) is pierced with two rods. The two rods, both of diameter 2 mm, are placed 8 mm and 2 mm transversely away from the centerline, and are 65 mm vertically staggered from each other. The mean flow in each panel is from top to bottom; from left to right the panels document the downstream evolution of the flow: $x/w \approx$ 10–14 (a), 15–19 (b), 20–24 (c) and 25–29 (d).

[1] W. K. George Jr, P. D. Beuther, and J. L. Lumley, in *Proceedings of the Dynamic Flow Conference 1978 on Dynamic Measurements in Unsteady Flows* (Springer, 1978) pp. 757–800.

[2] R. Adrian and C. Yao, Exp. Fluids **5**, 17 (1986).

[3] P. Vorobieff, M. Rivera, and R. E. Ecke, Phys. Fluids **11**, 2167 (1999).

[4] G. Boffetta and R. E. Ecke, Annu. Rev. Fluid Mech. **44**, 427 (2012).

[5] G. Comte-Bellot and S. Corrsin, J. Fluid Mech. **25**, 657 (1966).

[6] G. Boffetta and S. Musacchio, Phys. Rev. E **82**, 016307 (2010).

[7] M. K. Rivera, H. Aluie, and R. E. Ecke, Phys. Fluids **26**, 055105 (2014).
